# Supplementary material for: Quantum chemistry with Coulomb Sturmians: Construction and convergence of Coulomb Sturmian basis sets at Hartree-Fock level
Source: arXiv:1811.05777 ancillary file (2019-01-04)
Supplement: Supplementary file 1 [file supporting_info.pdf]

# Quantum chemistry with Coulomb Sturmians: Construction and convergence of Coulomb Sturmian basis sets at Hartree-Fock level

## Supporting information

Michael F. Herbst, James E. Avery, Andreas Dreuw

| system | CS basis | $k_{\text{opt}}$ | $N_{\text{bas}}$ | $E_{\text{HF}}$ | relative error |
|---|---|---|---|---|---|
| Li | $(4,1,1)$ | 1.56 | 13 | $-7.38483^{U}$ | $6.4 \cdot 10^{-03}$ |
| Li | $(5,1,1)$ | 1.54 | 17 | $-7.41652^{U}$ | $2.2 \cdot 10^{-03}$ |
| Li | $(6,1,1)$ | 1.53 | 21 | $-7.42812^{U}$ | $6.2 \cdot 10^{-04}$ |
| Be | $(4,1,1)$ | 2.02 | 13 | $-14.46796^{R}$ | $7.2 \cdot 10^{-03}$ |
| Be | $(5,1,1)$ | 1.99 | 17 | $-14.53916^{R}$ | $2.3 \cdot 10^{-03}$ |
| Be | $(6,1,1)$ | 1.99 | 21 | $-14.56445^{R}$ | $5.9 \cdot 10^{-04}$ |
| B | $(3,2,2)$ | 2.48 | 14 | $-23.64847^{U}$ | $3.6 \cdot 10^{-02}$ |
| B | $(4,1,1)$ | 2.46 | 13 | $-24.32117^{U}$ | $8.7 \cdot 10^{-03}$ |
| B | $(4,2,2)$ | 2.47 | 23 | $-24.32594^{U}$ | $8.5 \cdot 10^{-03}$ |
| B | $(5,1,1)$ | 2.43 | 17 | $-24.46411^{U}$ | $2.8 \cdot 10^{-03}$ |
| B | $(5,2,2)$ | 2.43 | 32 | $-24.46852^{U}$ | $2.6 \cdot 10^{-03}$ |
| B | $(6,1,1)$ | 2.41 | 21 | $-24.51204^{U}$ | $8.7 \cdot 10^{-04}$ |
| B | $(7,2,2)$ | 2.40 | 50 | $-24.52731^{U}$ | $2.5 \cdot 10^{-04}$ |
| C | $(4,1,1)$ | 2.92 | 13 | $-37.34490^{U}$ | $9.3 \cdot 10^{-03}$ |
| C | $(5,1,1)$ | 2.87 | 17 | $-37.58533^{U}$ | $2.9 \cdot 10^{-03}$ |
| C | $(6,1,1)$ | 2.85 | 21 | $-37.66284^{U}$ | $8.2 \cdot 10^{-04}$ |
| N | $(4,1,1)$ | 3.36 | 13 | $-53.88221^{U}$ | $9.6 \cdot 10^{-03}$ |
| N | $(5,1,1)$ | 3.32 | 17 | $-54.24940^{U}$ | $2.9 \cdot 10^{-03}$ |
| N | $(6,1,1)$ | 3.29 | 21 | $-54.36501^{U}$ | $7.3 \cdot 10^{-04}$ |
| O | $(5,2,2)$ | 3.74 | 32 | $-74.57763^{U}$ | $3.2 \cdot 10^{-03}$ |
| O | $(6,1,1)$ | 3.69 | 21 | $-74.74979^{U}$ | $9.3 \cdot 10^{-04}$ |
| O | $(7,2,2)$ | 3.64 | 50 | $-74.79613^{U}$ | $3.1 \cdot 10^{-04}$ |
| F | $(5,2,2)$ | 4.16 | 32 | $-99.07686^{U}$ | $3.4 \cdot 10^{-03}$ |
| F | $(6,1,1)$ | 4.10 | 21 | $-99.32043^{U}$ | $9.7 \cdot 10^{-04}$ |
| F | $(7,2,2)$ | 4.04 | 50 | $-99.38482^{U}$ | $3.2 \cdot 10^{-04}$ |
| Ne | $(4,1,1)$ | 4.64 | 13 | $-127.0528^{R}$ | $1.2 \cdot 10^{-02}$ |
| Ne | $(5,1,1)$ | 4.58 | 17 | $-128.0943^{R}$ | $3.5 \cdot 10^{-03}$ |
| Ne | $(6,1,1)$ | 4.51 | 21 | $-128.4255^{R}$ | $9.5 \cdot 10^{-04}$ |

$^{U}$ unrestricted HF
$^{R}$ restricted HF

Table SI-1: Optimal CS exponent for the 2nd period of the periodic table at HF level. Relative errors are given with respect to the reference energies of table I shown in the main text.

| system | CS basis | $k_{\text{opt}}$ | $N_{\text{bas}}$ | $E_{\text{HF}}$ | relative error |
|---|---|---|---|---|---|
| Na | $(5,1,1)$ | 4.45 | 17 | $-159.8132^U$ | $1.3 \cdot 10^{-02}$ |
| Na | $(6,1,1)$ | 4.29 | 21 | $-160.9291^U$ | $5.7 \cdot 10^{-03}$ |
| Na | $(7,1,1)$ | 4.10 | 25 | $-161.4028^U$ | $2.8 \cdot 10^{-03}$ |
| Na | $(8,1,1)$ | 3.92 | 29 | $-161.6200^U$ | $1.5 \cdot 10^{-03}$ |
| Mg | $(5,1,1)$ | 4.58 | 17 | $-196.1362^R$ | $1.7 \cdot 10^{-02}$ |
| Mg | $(6,1,1)$ | 4.44 | 21 | $-198.0276^R$ | $8.0 \cdot 10^{-03}$ |
| Mg | $(7,1,1)$ | 4.27 | 25 | $-198.8705^R$ | $3.7 \cdot 10^{-03}$ |
| Mg | $(8,1,1)$ | 4.11 | 29 | $-199.2445^R$ | $1.9 \cdot 10^{-03}$ |
| Al | $(6,2,2)$ | 4.65 | 41 | $-239.5138^U$ | $9.8 \cdot 10^{-03}$ |
| Al | $(7,1,1)$ | 4.48 | 25 | $-240.7812^U$ | $4.5 \cdot 10^{-03}$ |
| Al | $(7,2,2)$ | 4.49 | 50 | $-240.7885^U$ | $4.5 \cdot 10^{-03}$ |
| Si | $(5,2,2)$ | 5.01 | 32 | $-282.0009^U$ | $2.4 \cdot 10^{-02}$ |
| Si | $(6,2,2)$ | 4.90 | 41 | $-285.7755^U$ | $1.1 \cdot 10^{-02}$ |
| Si | $(7,1,1)$ | 4.75 | 25 | $-287.4682^U$ | $4.8 \cdot 10^{-03}$ |
| Si | $(7,2,2)$ | 4.75 | 50 | $-287.4751^U$ | $4.8 \cdot 10^{-03}$ |
| Si | $(8,1,1)$ | 4.62 | 29 | $-288.1995^U$ | $2.3 \cdot 10^{-03}$ |
| P | $(6,1,1)$ | 5.19 | 21 | $-336.9464^U$ | $1.1 \cdot 10^{-02}$ |
| P | $(7,1,1)$ | 5.05 | 25 | $-339.0724^U$ | $4.8 \cdot 10^{-03}$ |
| P | $(8,1,1)$ | 4.92 | 29 | $-339.9651^U$ | $2.2 \cdot 10^{-03}$ |
| S | $(5,2,2)$ | 5.54 | 32 | $-387.1635^U$ | $2.6 \cdot 10^{-02}$ |
| S | $(6,2,2)$ | 5.48 | 41 | $-392.9687^U$ | $1.1 \cdot 10^{-02}$ |
| S | $(7,2,2)$ | 5.35 | 50 | $-395.5575^U$ | $4.9 \cdot 10^{-03}$ |
| Cl | $(5,2,2)$ | 5.82 | 32 | $-447.2744^U$ | $2.7 \cdot 10^{-02}$ |
| Cl | $(6,2,2)$ | 5.78 | 41 | $-454.1715^U$ | $1.2 \cdot 10^{-02}$ |
| Cl | $(7,2,2)$ | 5.66 | 50 | $-457.2387^U$ | $4.9 \cdot 10^{-03}$ |
| Ar | $(5,1,1)$ | 6.11 | 17 | $-512.6726^R$ | $2.7 \cdot 10^{-02}$ |
| Ar | $(6,1,1)$ | 6.08 | 21 | $-520.7125^R$ | $1.2 \cdot 10^{-02}$ |
| Ar | $(7,1,1)$ | 5.97 | 25 | $-524.2770^R$ | $4.8 \cdot 10^{-03}$ |
| Ar | $(8,1,1)$ | 5.86 | 29 | $-525.7054^R$ | $2.1 \cdot 10^{-03}$ |

$^U$ unrestricted HF
$^R$ restricted HF

Table SI-2: Optimal CS exponent for the 3rd period of the periodic table at HF level. Relative errors are given with respect to the reference energies of table I shown in the main text.
